# Supplementary material for: Aligning Latent and Image Spaces to Connect the Unconnectable
Source: arXiv:2104.06954 source file (2021-04-14)
Supplement: Supplementary file 1 [file periodic-positional-embeddings.tex]

\section{Several remarks on periodic positional embeddings}\label{ap:periodic-pos-embs}

TODO: figures for log-linear and SIREN

TODO: Compare in terms of number of parameters

TODO: ablations for log-linear with local vs log-linear with global vs siren with small amount vs siren with large amount of channels
